# Supplementary material for: SldprtNet: A Large-Scale Multimodal Dataset for CAD Generation in Language-Driven 3D Design
Source: arXiv:2603.13098 source file (2026-03-13)
Supplement: Supplementary file 1 [file Appendix.tex]

\section*{APPENDIX}
